# Supplementary material for: Collective magnetic splitting in single-photon superradiance
Source: arXiv:1606.02988 source file (2016-07-22)
Supplement: Supplementary file 1 [file SupplementaryMaterial.pdf]

# Collective Magnetic Splitting in Single-Photon Superradiance: Supplemental Material

Xiangjin Kong and Adriana Pálffy

Max-Planck-Institut für Kernphysik, Saupfercheckweg 1, 69117 Heidelberg, Germany

In the following we present in detail the more involved analytic derivation of the expressions presented in the main text.

## EIGENVALUE EXPRESSIONS

As starting point we take the Schrödinger equation (setting $\hbar = 1$)

$$|\dot{\psi}(t)\rangle = -iH_{int}|\psi(t)\rangle\,. \tag{S1}$$

for the system composed of atoms and the field in a superposition of Fock states as presented in Eq. (2) in the main text. Substituting Eqs. (1) and (2) into Eq. (S1) and integrating over time with the initial conditions $\gamma_k(0) = 0$ and $\alpha_k^{mn}(0) = 0$, we obtain the following equation for $\beta_1^j(t)$

$$\begin{aligned}
\frac{\partial \beta_1^j(t)}{\partial t} = & -\sum_{\vec{k}}\sum_{j'=1}^{N_1}\int_0^t dt' g_k^2 \beta_1^{j'}(t') e^{i(\nu_k-\omega_1)(t'-t)+i\vec{k}\cdot(\vec{r}_j-\vec{r}_{j'})} \\
& -(N_1-1)\sum_{\vec{k}}\int_0^t dt' g_k^2 \beta_1^{j'}(t') e^{i(\nu_k+\omega_1)(t'-t)} \\
& -\sum_{\vec{k}}\sum_{j'=1,j'\neq j}^{N_1}\int_0^t dt' g_k^2 \beta_1^{j'}(t') e^{i(\nu_k+\omega_1)(t'-t)-i\vec{k}\cdot(\vec{r}_j-\vec{r}_{j'})} \\
& -\sum_{\vec{k}}\sum_{j'=N_1+1}^{N}\int_0^t dt' g_k^2 \beta_2^{j'}(t') e^{i(\nu_k-\omega_2)t'-i(\nu_k-\omega_1)t+i\vec{k}\cdot(\vec{r}_j-\vec{r}_{j'})} \\
& -(N-N_1)\sum_{\vec{k}}\int_0^t dt' g_k^2 \beta_2^{j'}(t') e^{i(\nu_k+\omega_2)(t'-t)} \\
& -\sum_{\vec{k}}\sum_{j'=N_1+1}^{N}\int_0^t dt' g_k^2 \beta_2^{j'}(t') e^{i(\nu_k+\omega_1)t'-i(\nu_k+\omega_2)t-i\vec{k}\cdot(\vec{r}_j-\vec{r}_{j'})}\,.
\end{aligned} \tag{S2}$$

The first three terms of the expression above can be condensed following Ref. [11] to

$$-\gamma\beta_1^j(t) + i\gamma\sum_{j'\neq j,j'=1}^{N_1}\frac{\exp(k_0|r_j-r_{j'}|)}{k_0|\vec{r}_j-\vec{r}_{j'}|}\beta_1^{j'}(t)\,, \tag{S3}$$

where $k_0 = \frac{\omega_1+\omega_2}{2c}$ and $c$ is the speed of light in vacuum. The remaining part of Eq. (S2) is simplified under the assumption that $e^{i(\omega_1-\omega_2)t'} \simeq e^{i(\omega_1-\omega_2)t}$ which is valid provided the state decay time is much larger than the time of photon flight through the atomic cloud to yield

$$i\gamma e^{i\phi t} \sum_{j'=N_1+1}^{N} \frac{\exp(ik_0|\vec{r}_j - \vec{r}_{j'}|)}{k_0|\vec{r}_j - \vec{r}_{j'}|} \beta_2^{j'}(t)\,, \tag{S4}$$

where $\phi = \omega_1 - \omega_2$. The Schrödinger equation for $\beta_1^j(t)$ then reads in this simplified form

$$\frac{\partial \beta_1^j(t)}{\partial t} = -\gamma \beta_1^j(t) + i\gamma \sum_{j'\neq j, j'=1}^{N_1} \frac{\exp(ik_0|\vec{r}_j - \vec{r}_{j'}|)}{k_0|\vec{r}_j - \vec{r}_{j'}|} \beta_1^{j'}(t)$$

$$+ i\gamma e^{i\phi t} \sum_{j'=N_1+1}^{N} \frac{\exp(ik_0|\vec{r}_j - \vec{r}_{j'}|)}{k_0|\vec{r}_j - \vec{r}_{j'}|} \beta_2^{j'}(t)\,. \tag{S5}$$

We perform a similar simplification for $\beta_2^j(t)$ and obtain

$$\frac{\partial \beta_2^j(t)}{\partial t} = -\gamma \beta_2^j(t) + i\gamma \sum_{j'\neq j,, j'=N_1+1}^{N} \frac{\exp(ik_0|\vec{r}_j - \vec{r}_{j'}|)}{k_0|\vec{r}_j - \vec{r}_{j'}|} \beta_2^{j'}(t)$$

$$+ i\gamma e^{-i\phi t} \sum_{j'=1}^{N_1} \frac{\exp(ik_0|\vec{r}_j - \vec{r}_{j'}|)}{k_0|\vec{r}_j - \vec{r}_{j'}|} \beta_1^{j'}(t)\,. \tag{S6}$$

Next we assume that initially the system is prepared in an eigenstate,

$$\beta_1^j(t) = \beta_1^j e^{(-\lambda_n + \frac{i}{2}\phi)t},\ \beta_2^j(t) = \beta_2^j e^{(-\lambda_n - \frac{i}{2}\phi)t}\,, \tag{S7}$$

where $\lambda_n$ is the eigenvalue and we choose $\mathrm{Re}(\lambda_n) > 0$ following Ref. [11]. Substituting Eq. (S7) into Eqs. (S5) and (S6) yields the following eigenvalue equations:

$$\left(-\lambda_n + \frac{i}{2}\phi\right)\beta_1^j = -\gamma \beta_1^j + i\gamma \sum_{j'\neq j, j'=1}^{N_1} \frac{\exp(ik_0|\vec{r}_j - \vec{r}_{j'}|)}{k_0|\vec{r}_j - \vec{r}_{j'}|} \beta_1^{j'}$$

$$+ i\gamma \sum_{j'=N_1+1}^{N} \frac{\exp(ik_0|\vec{r}_j - \vec{r}_{j'}|)}{k_0|\vec{r}_j - \vec{r}_{j'}|} \beta_2^{j'}\,, \tag{S8}$$

$$\left(-\lambda_n - \frac{i}{2}\phi\right)\beta_2^j = -\gamma \beta_2^j + i\gamma \sum_{j'\neq j,, j'=N_1+1}^{N} \frac{\exp(ik_0|\vec{r}_j - \vec{r}_{j'}|)}{k_0|\vec{r}_j - \vec{r}_{j'}|} \beta_2^{j'}$$

$$+ i\gamma \sum_{j'=1}^{N_1} \frac{\exp(ik_0|\vec{r}_j - \vec{r}_{j'}|)}{k_0|\vec{r}_j - \vec{r}_{j'}|} \beta_1^{j'}\,. \tag{S9}$$

For a dense cloud with many atoms in the volume $\lambda^3$ ($\lambda = 2\pi c/\omega_0$) one can go to the continuous limit and replace the summation over $j'$ by integration. We should notice that in the summation we divide the atoms into two "teams" depending on the transitions that they undergo. The integration is performed over the entire sample volume, with the atoms of the two "teams" distributed across the latter, and their densities reduced by a factor $1/2$ if we consider $N_1 \approx N/2$. Then, the eigenvalue equations (S8) and (S9) read in integral form

$$\left(-\lambda_n + \frac{i}{2}\phi\right)\beta_1(\vec{r}) = -\frac{\gamma}{2}\beta_1(\vec{r}) + i\gamma\int \frac{\exp(ik_0|\vec{r}-\vec{r}'|)}{k_0|\vec{r}-\vec{r}'|}\beta_1(\vec{r}')\rho_1(\vec{r}')d\vec{r}$$

$$+\frac{\gamma}{2}\beta_2(\vec{r}) + i\gamma\int \frac{\exp(ik_0|\vec{r}-\vec{r}'|)}{k_0|\vec{r}-\vec{r}'|}\beta_2(\vec{r}')\rho_2(\vec{r}')d\vec{r}, \tag{S10}$$

$$\left(-\lambda_n - \frac{i}{2}\phi\right)\beta_2(\vec{r}) = -\frac{\gamma}{2}\beta_2(\vec{r}) + i\gamma\int \frac{\exp(ik_0|\vec{r}-\vec{r}'|)}{k_0|\vec{r}-\vec{r}'|}\beta_2(\vec{r}')\rho_2(\vec{r}')d\vec{r}$$

$$+\frac{\gamma}{2}\beta_1(\vec{r}) + i\gamma\int \frac{\exp(ik_0|\vec{r}-\vec{r}'|)}{k_0|\vec{r}-\vec{r}'|}\beta_1(\vec{r}')\rho_1(\vec{r}')d\vec{r}, \tag{S11}$$

where $\rho_1(r) = \rho_2(r) = \frac{N}{2V}$. After some further simplifications, we obtain

$$\frac{i}{2}\phi\,[\beta_1(\vec{r}) + \beta_2(\vec{r})] = (\lambda_n - \gamma)\,[\beta_1(\vec{r}) - \beta_2(\vec{r})]\,, \tag{S12}$$

$$\left(\lambda_n + \frac{\phi^2}{4(\lambda_n-\gamma)}\right)[\beta_1(\vec{r}) + \beta_2(\vec{r})] = -i\gamma\frac{N}{V} \times \int \frac{\exp(ik_0|\vec{r}-\vec{r}'|)}{k_0|\vec{r}-\vec{r}'|}\left[\beta_1(\vec{r}') + \beta_2(\vec{r}')\right]d\vec{r}'. \tag{S13}$$

We introduce the notations

$$\beta(\vec{r}) = \beta_1(\vec{r}) + \beta_2(\vec{r})\,, \tag{S14}$$

and

$$\lambda_n' = \lambda_n + \frac{\phi^2}{4(\lambda_n-\gamma)}\,. \tag{S15}$$

Substituting Eqs. (S14) and (S15) into Eq. (S13) yields

$$\lambda_n'\beta(\vec{r}) = -i\gamma\frac{N}{V}\int d\vec{r}'\frac{\exp(ik_0|\vec{r}-\vec{r}'|)}{k_0|\vec{r}-\vec{r}'|}\beta(\vec{r}')\,. \tag{S16}$$

We find that Eq. (S16) has the same expression as the eigenvalue equation in the two-level system [11] for $\lambda_n'$. Thus, we find that $\lambda_n'$ is actually the eigenvalue of the system in the absence of the magnetic field. We write the solution in the complex form $\lambda_n' = \Gamma + i\mathscr{L}$, where the real part $\Gamma$ stands for the superradiant decay rate and the imaginary part $\mathscr{L}$ represents the collective Lamb

shift of the system of $N$ two-level atoms without any magnetic field. Based on these expressions, the eigenvalues of the system in the presence of the magnetic field splitting can be obtained [Eq. (3) in the main text]:

$$\lambda_{\pm} = \frac{\Gamma + \gamma + i\mathscr{L} \mp i\sqrt{\phi^2 + [\mathscr{L} - i(\Gamma - \gamma)]^2}}{2}. \tag{S17}$$

**THE RADIATION SPECTRUM**

If the system is prepared initially in an excited eigenstate, we can obtain the spectrum of the radiation photon from the corresponding Schrödinger equation Eq. (S1)

$$\begin{aligned}\frac{\partial \gamma_{\vec{k}}}{\partial t} = &- i g_k \int d\vec{r}' \rho_1(\vec{r}')\beta_1(\vec{r}')e^{-\lambda_n + i(\nu_k + \frac{\phi}{2} - \omega_1)t - i\vec{k}\cdot\vec{r}'} \\ &- i g_k \int d\vec{r}' \rho_2(\vec{r}')\beta_2(\vec{r}')e^{-\lambda_n + i(\nu_k - \frac{\phi}{2} - \omega_2)t - i\vec{k}\cdot\vec{r}'}.\end{aligned} \tag{S18}$$

For the case of an uniformly excited sample considering the initial condition

$$\beta_1^j + \beta_2^j = \sqrt{\frac{1}{N}} e^{i\vec{k}_0\cdot\vec{r}_j}, \;\; j = 1, 2....N, \tag{S19}$$

we obtain

$$\gamma_{\vec{k}} = \sqrt{N} g_k \frac{1 - e^{i(\nu_k - \omega_0)t - \lambda_n t}}{(\nu_k - \omega_0) + i\lambda_n} \frac{\int d\vec{r}' e^{i(\vec{k}_0 - \vec{k})\cdot\vec{r}'}}{V}. \tag{S20}$$

In the following we pay attention to the limit $R \ll \lambda$, for which we can approximate

$$e^{i(\vec{k}_0 - \vec{k})\cdot\vec{r}'} \approx e^{i(\vec{k}_0 - \vec{k})\cdot\vec{r}_0}, \tag{S21}$$

where $\vec{r}_0$ is the central position of the atoms. With this approximation we find

$$\gamma_{\vec{k}} = \sqrt{N} g_k e^{i(\vec{k}_0 - \vec{k})\cdot\vec{r}_0} \frac{1 - e^{i(\nu_k - \omega_0)t - \lambda_n t}}{(\nu_k - \omega_0) + i\lambda_n}. \tag{S22}$$

In the more general case considered in the main text, the initial state of the system is not in an eigenstate, but in a mixed state reached by the excitation from both ground states to

$$\begin{aligned}|\psi_1\rangle &= \frac{1}{\sqrt{N/2}} \sum_{j=1}^{N/2} e^{i\vec{k}_0\cdot\vec{r}_j} |g_1 g_2 ... e_j ... g_{N/2} ... g_N\rangle |0\rangle, \\ |\psi_2\rangle &= \frac{1}{\sqrt{N/2}} \sum_{j=N/2+1}^{N} e^{i\vec{k}_0\cdot\vec{r}_j} |g_1 ... g_{N/2} g_{N/2+1} ... e_j ... g_N\rangle |0\rangle.\end{aligned} \tag{S23}$$

We assume that initially the system is in a mixed state which has a 50% probability to be in state $|\psi_1\rangle$ or in state $|\psi_2\rangle$, respectively. We mark the two eigenstates of the system as $|E_+\rangle$ and $|E_-\rangle$, corresponding to the eigenvalues $\lambda_+$ and $\lambda_-$,

$$|E_+\rangle = \sum_{j=1}^{N/2} \beta_{1+}^{j}(t)|g_1 g_2 ... e_j ... g_{N/2} ... g_N\rangle|0\rangle + \sum_{j=N/2+1}^{N} \beta_{2+}^{j}(t)|g_1 ... g_{N/2} g_{N/2+1} ... e_j ... g_N\rangle|0\rangle\,, \quad \text{(S24)}$$

$$|E_-\rangle = \sum_{j=1}^{N/2} \beta_{1-}^{j}(t)|g_1 g_2 ... e_j ... g_{N/2} ... g_N\rangle|0\rangle + \sum_{j=N/2+1}^{N} \beta_{2-}^{j}(t)|g_1 ... g_{N/2} g_{N/2+1} ... e_j ... g_N\rangle|0\rangle\,. \quad \text{(S25)}$$

Let us now assume that the system has a probability $a$ to be at $t = 0$ in the eigenstate $|E_+\rangle$. From Eqs. (S14)–(S16) we obtain

$$\beta_{1+}(r) + \beta_{2+}(r) = \beta_{1-}(r) + \beta_{2-}(r) = \sqrt{\frac{1}{N}} e^{i\vec{k}_0 \cdot \vec{r}}\,. \quad \text{(S26)}$$

From Eq. (S12) we find that

$$[\beta_{1+}(r) - \beta_{2+}(r)] = \frac{i\phi}{2(\lambda_+ - \gamma)} [\beta_{1+}(r) + \beta_{2+}(r)]\,, \quad \text{(S27)}$$

$$[\beta_{1-}(r) - \beta_{2-}(r)] = \frac{i\phi}{2(\lambda_- - \gamma)} [\beta_{1-}(r) + \beta_{2-}(r)]\,. \quad \text{(S28)}$$

Finally the initial condition $\beta_1(r) = \beta_2(r)$ translates into

$$a\beta_{1+}(r) + (1-a)\beta_{1-}(r) = a\beta_{2+}(r) + (1-a)\beta_{2+}(r)\,. \quad \text{(S29)}$$

Combining the results above we then can derive that

$$\left[a\frac{i\phi}{2(\lambda_+ - \gamma)} + (1-a)\frac{i\phi}{2(\lambda_- - \gamma)}\right] [\beta_{1+}(r) + \beta_{2+}(r)] = 0\,, \quad \text{(S30)}$$

and

$$a\frac{i\phi}{2(\lambda_+ - \gamma)} + (1-a)\frac{i\phi}{2(\lambda_- - \gamma)} = 0\,. \quad \text{(S31)}$$

The probability for the system to be intially in the eigenstate $|E_+\rangle$ thus reads

$$a = \frac{\lambda_+ - \gamma}{\lambda_+ - \lambda_-}\,. \quad \text{(S32)}$$

We turn now to the emitted radiation. Taking into account Eq. (S22) we find in this case

$$\gamma_{\vec{k}} = \sqrt{N} g_k e^{i(\vec{k}_0 - \vec{k})\cdot\vec{r}_0} \left( \frac{\lambda_+ - \gamma}{\lambda_+ - \lambda_-} \frac{1 - e^{i(\nu_k - \omega_0)t - \lambda_+ t}}{(\nu_k - \omega_0) + i\lambda_+} - \frac{\lambda_- - \gamma}{\lambda_+ - \lambda_-} \frac{1 - e^{i(\nu_k - \omega_0)t - \lambda_- t}}{(\nu_k - \omega_0) + i\lambda_-} \right). \tag{S33}$$

Upon introducing the field state [32] we reproduce Eq. (4) in the main text,

$$|\gamma_0\rangle = \sum_{\vec{k}} \sqrt{N} g_k e^{i(\vec{k}_0 - \vec{k})\cdot\vec{r}_0} \left( \frac{A_+}{\nu_k - \omega_0 + i\lambda_+} + \frac{A_-}{\nu_k - \omega_0 + i\lambda_-} \right) |1_{\vec{k}}\rangle , \tag{S34}$$

where $A_\pm = \pm(\lambda_\pm - \gamma)/(\lambda_+ - \lambda_-)$. This is a linear superposition of single-photon states with different corresponding wave vectors. For long times compared to the superradiance decay $t \gg \Gamma^{-1}$, the system evolves into $|\psi(t)\rangle \to |g_1 g_2 ... g_N\rangle|\gamma_0\rangle$. Here the index '0' in $|\gamma_0\rangle$ reminds that this state corresponds to the situation when all atoms can be considered located at position $r_0$ in the limit of $R \ll \lambda$.
